# Supplementary material for: Next-to-Leading-Order Corrections to Weak Boson Production with a Massive Quark Jet Pair at Hadron Colliders
Source: arXiv:0809.3829 source file (2008-09-23)
Supplement: Supplementary file 1 [file appendixRen.tex]

%%%%%%%%%%%%%%%%%%%%%%%%%%%%%%%%%%%%%%%%%%%%%%%%%%%%%%%%%%%%%%%%%%%%%%%
\chapter{Renormalization}\label{app:Renom}

%%%%%%%%%%%%%%%%%%%%%%%%%%%%%%%%%%%%%%%%%%%%%%%%%%%%%%%%%%%%%%%%%%%%%%%
how to hide the infinities under the rug...

\endinput
